# Supplementary material for: Universal Critical Jump for Inverse-Square Ising Ferromagnets
Source: arXiv:2610.36131 source file (2026-10-26)
Supplement: Supplementary file 2 [file supplement_macros.tex]

\newcommand{\E}{\mathbb E}
\newcommand{\Pp}{\mathbb P}
\newcommand{\R}{\mathbb R}
\newcommand{\N}{\mathbb N}
\newcommand{\C}{\mathbb C}
\newcommand{\dd}{\mathrm d}
\newcommand{\ind}{\mathbf1}
\newcommand{\norm}[1]{\lVert#1\rVert}
\newcommand{\ip}[2]{\langle#1,#2\rangle}
\newcommand{\calH}{\mathcal H}
\newcommand{\calE}{\mathcal E}
\newcommand{\calO}{\mathcal O}
\newcommand{\calT}{\mathcal T}
\DeclareMathOperator{\Tr}{Tr}
\DeclareMathOperator{\Var}{Var}
\DeclareMathOperator{\Cov}{Cov}
\DeclareMathOperator{\Ent}{Ent}
\DeclareMathOperator{\KL}{KL}
\DeclareMathOperator{\supp}{supp}
\DeclareMathOperator{\spec}{spec}
\DeclareMathOperator{\TV}{TV}
\DeclareMathOperator{\clip}{clip}
